# Supplementary material for: Time Series Methods and Ensemble Models to Nowcast Dengue at the State Level in Brazil
Source: arXiv:2006.02483 source file (2020-06-03)
Supplement: Supplementary file 1 [file 7-additional_information.tex]

\section*{Additional information}

\instructions{To include, in this order: \textbf{Accession codes} (where applicable); \textbf{Competing financial interests} (mandatory statement). The corresponding author is responsible for submitting a competing financial interests statement on behalf of all authors of the paper. This statement must be included in the submitted article file.}
